# Supplementary material for: GID: Graph-based Intrusion Detection on Massive Process Traces for Enterprise Security Systems
Source: arXiv:1608.02639 source file (2016-08-08)
Supplement: Supplementary file 1 [file SDM2016_GID_SupplementaryFile.pdf]

# Supplementary Document for GID: Graph-based Intrusion Detection Using Process Traces

Boxiang Dong\*    Zhenzhang Chen<sup>†</sup>    Hui (Wendy) Wang\*    Lu-an Tang<sup>†</sup>    Kai Zhang<sup>†</sup>  
 Ying Lin<sup>‡</sup>    Haifeng Chen<sup>†</sup>    Guofei Jiang<sup>†</sup>

October 16, 2015

| Symbol        | Description                                           |
|---------------|-------------------------------------------------------|
| $n_b$         | The source entity of an event                         |
| $n_d$         | The destination entity of an event                    |
| $\mathcal{E}$ | System monitoring data containing events              |
| $\mathcal{B}$ | A set of valid event sequence patterns                |
| $\mathcal{C}$ | The set of candidate paths                            |
| $\mathcal{S}$ | The set of suspicious paths                           |
| $\mathcal{A}$ | The set of abnormal event sequences                   |
| $G$           | The multipartite graph constructed from $\mathcal{E}$ |
| $\Delta t$    | The time window size                                  |
| $P$           | The set of process nodes in $G$                       |
| $F$           | The set of file nodes in $G$                          |
| $U$           | The set of UDSocket nodes in $G$                      |
| $I$           | The set of INETSocket nodes in $G$                    |
| $B$           | A event sequence pattern                              |
| $ B $         | The number of different entity types in $B$           |
| $p$           | A path in $G$                                         |

Table 1: Notations

| Entity     | Attributes                                                      |
|------------|-----------------------------------------------------------------|
| Process    | process_id, user_id, process_path                               |
| File       | volume_id, data_id, user_id, file_path                          |
| INETSocket | inet_id, local_ip, local_port, destination_ip, destination_port |
| UDSocket   | ud_id, source_path, destination_path                            |

Table 2: Attributes of System Entities

| Type                                  | Number |
|---------------------------------------|--------|
| $\langle Process, File \rangle$       | 340M   |
| $\langle Process, Process \rangle$    | 350K   |
| $\langle Process, INETSocket \rangle$ | 170K   |
| $\langle Process, UDSocket \rangle$   | 440K   |
| $\langle UDSocket, UDSocket \rangle$  | 30K    |

Table 3: Number of interactions between different system entities

## 1 Notations

In Table 1, we list the notations we use in this paper.

## 2 Entity Attributes

In Section 2 of the paper, we explain the system entities that appear in the system monitoring data. Basically, there are four types of system entities: (1) *files*, (2) *processes*, (3) *Unix domain sockets* (UDSockets), and (4) *Internet sockets* (INETSockets). Each type of entities is associated with a set of attributes. The entity attributes are shown in Table 2.

## 3 Suspicious Path Validation

The discovered top- $k$  suspicious paths are not necessarily related to intrusion attacks to the computer system, unless they are sufficiently distinctive from those normal paths (we take the remaining paths that are not top- $k$  ranked as normal). To further validate the discovered suspicious paths, we calculate the  $t$ -value between the two groups of paths: all candidate paths  $\mathcal{C}$ , and the set of discovered suspicious paths  $\mathcal{S}$ .

Formally, let  $\mathcal{C}$  denote all the candidate paths,  $\mathcal{S}$  the set of discovered suspicious paths, and  $\mathcal{N} = \mathcal{C} - \mathcal{S}$ . Formally, the  $t$ -value  $t$  is

$$(3.1) \quad t = \frac{E_{\mathcal{S}} - E_{\mathcal{N}}}{\sqrt{\frac{Var_{\mathcal{S}}}{|\mathcal{S}|} + \frac{Var_{\mathcal{N}}}{|\mathcal{N}|}}},$$

where  $E_{\mathcal{S}}$  ( $E_{\mathcal{N}}$ ) and  $Var_{\mathcal{S}}$  ( $Var_{\mathcal{N}}$ ) are defined below.

\*Department of Computer Science, Stevens Institute of Technology, NJ 07030

<sup>†</sup>NEC Laboratories, America Inc., Princeton, NJ 08540

<sup>‡</sup>University of Washington, Seattle, WA 98195

$$(3.2) \quad E_S = \frac{\sum_{p \in \mathcal{S}} \text{susp}(p)}{|\mathcal{S}|},$$

and

$$(3.3) \quad \text{VAR}_S = \sum_{p \in \mathcal{S}} (\text{susp}(p)^2 - E_S^2),$$

where

$$(3.4) \quad \text{susp}(p) = \mathcal{T}(\text{Score}(p), \lambda)$$

Equation 3.1 returns a confidence score that determines whether the difference between the two sets of paths is significant. If the confidence score is greater than a user-specified threshold, all paths in  $\mathcal{S}$  are considered as abnormal paths that are relevant to intrusion attacks. Otherwise, we treat those paths as normal and do not raise alerts.

#### 4 Graph Compactness

The performance of our intrusion detection method highly relies on our graph data structure. In this section, we measure the size of the constructed graph, aiming to show its compactness.

|      | Process | File   | INETSocket | UDSocket | Edge   |
|------|---------|--------|------------|----------|--------|
| Avg. | 117.3   | 191.36 | 0.93       | 41.42    | 1668.4 |
| Max  | 1468    | 23290  | 130        | 6735     | 58555  |

(a) Avg/max. number of nodes and edges

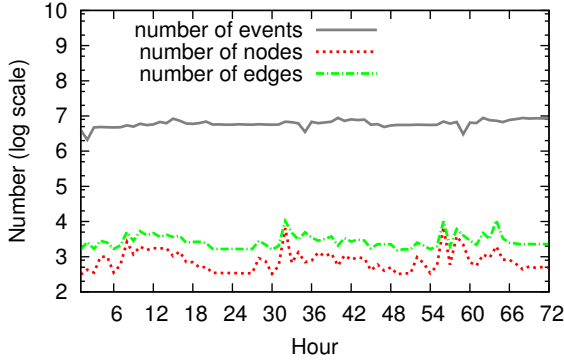

(b) Graph size vs. number of events

Figure 1: Graph compactness

In Figure 1 (a), we measure the size of our system log graph in terms of number of nodes and edges, and compare it with the number of events in the monitoring data. Specifically, we construct a graph per host per hour. Thus based on the monitoring data for 33 machines and 3 days, there are  $72 \times 33 = 2,376$  graphs.

In Figure 1 (a), we present the average and maximum size of the 2,376 graphs. On average, each graph contains 300 nodes and 1.6K edges. In Figure 1 (b), we show the average size of the graphs for each hour in a 72-hour time window. The number of nodes and edges are measured by averaging the size of the 33 graphs (for 33 hosts) in one hour. The results show that the graph can indeed reduce the space dramatically; around 340 millions of system events are represented by at most 2.5 million nodes and 4 million edges. The compact graph structure enables the efficient search for abnormal events. One interesting observation is that the graph reaches its largest size at the 10-th, 34-th and 58-th hour. These 3 peak hours correspond to the 10am of Day 1, Day 2 and Day 3 respectively. Normally 10am is the busiest time of system logging system as it is when most employees arrive at office.

#### 5 Distribution of Sender and Receiver Scores

In this section, we collect the distribution of our sender and receiver scores that are computed by the random walk approach (Section 3.5). The purpose of showing the distribution is to demonstrate that the anomaly score, which is computed from the sender and receiver scores, indeed catches the suspicious interactions between entities. We measure the *density distribution* that describes the probability that the sender/receiver score falls into a given range. In Figure 2 (a), we display the density distribution of the sender scores of one specific host. We only show the results of one host as all the hosts have similar score distribution. It can be seen that the sender scores are of a polarized distribution. We investigate the reason and find that many files such as shared libraries (e.g., *libpthread.so* and *libcrypt.so* files) and system configuration files (e.g., */etc/security/capability.conf* and */etc/security/limits.conf* files) are frequently accessed by various processes. Thus, the sender scores of these files are relatively high. There also exist daemon processes such as */bin/dbus-daemon* and user files that never function as a information sender. This explains why a large fraction of entities have low sender scores. Conversely, most system entities have a relatively low receiver score. This is because only a limited number of processes such as *cron* regularly scan files and result in high receiver scores. Meanwhile, A majority of system entities are files which are seldom updated, leading to the fact that a large portion of system entities have low receiver scores. Therefore, our sender and receiver score computations truly models the system behaviors.

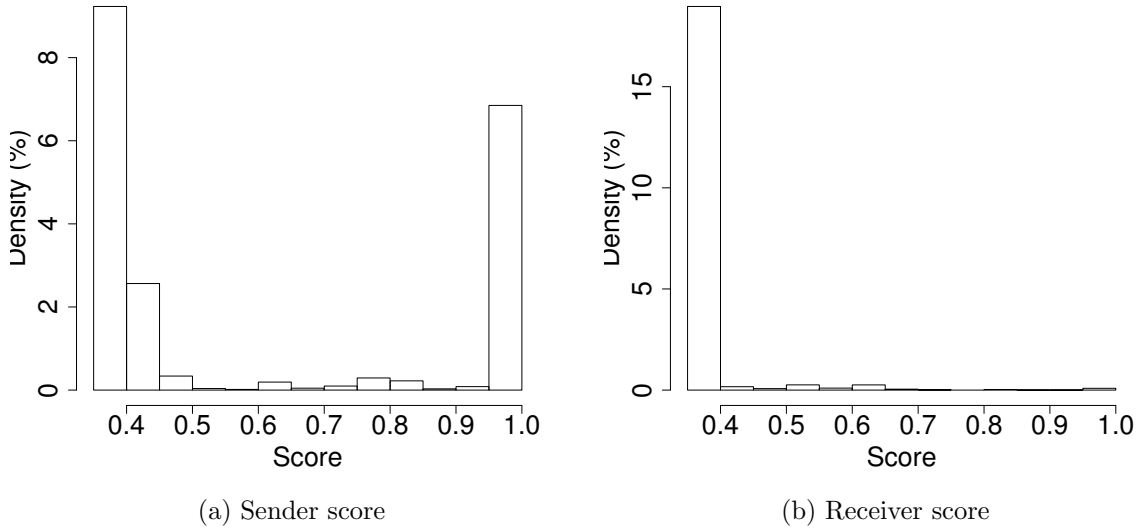

Figure 2: Sender and receiver score distribution

## 6 Some Other Related Work

**6.1 Meta-path** Meta-path could be considered as the closest approximation to the path pattern in the proposed method, especially, if the problem is to measure the relevance between two entities. Meta-path is a path that connects entity types via a sequence of relations. For example, given two types of entities: organization (O) and author (A), the meta-path A-O-A denotes the colleague relationship between two authors. With this meta-path, even though there is no direct link between two authors, we are able to measure their similarity/relationship based on the indirect links/paths. Meta-paths are popularly used for relevance search [2, 4, 5] and clustering [6].

Our event sequence pattern follows the same intuition of meta-path. But it is defined based on a sequence of entity types, rather than relations. Another major difference is that the event sequence is used as a guidance to search for candidate event sequences, instead of evaluating the relevance between two entities.

**6.2 Backtracking** Backtracking technique can also be used to analyze malicious process paths but it relies on a precise detection point, which is the state on the local computer system that alerts the user of the intrusion. Working back from a detection point (e.g., a suspicious file), BackTracker [1] identifies the chains of system events that could have led to the detected intrusion. Backtracking is also utilized to detect unwanted network traffic due to P2P address

misconfiguration [3]. In general, backtracking takes an accurate intrusion detection result as input and further searches for its evolvment processes. Our approach differs from backtracking in that the goal is to *real-time* detect the attack, not *offline* backtrack from the time when the attack happens.

Our approach differs from backtracking in that the goal is to detect the intrusion, which is of higher importance. On the other hand, to identify a reasonable number (30-50) of potential intrusion chains, backtracking must be deployed offline to conduct the analysis. In contrast, we are looking for a real-time intrusion detection solution.

## References

- [1] S. T. King et al. Backtracking intrusions. In *SIGOSP*, volume 37, pages 223–236, 2003.
- [2] S. Lee et al. Pathrank: a novel node ranking measure on a heterogeneous graph for recommender systems. In *CIKM*, pages 1637–1641, 2012.
- [3] Z. Li et al. Measurement and diagnosis of misconfigured peer-to-peer traffic. In *INFOCOM*, pages 1–9, 2010.
- [4] C. Shi et al. Relevance search in heterogeneous networks. In *EDBT*, pages 180–191, 2012.
- [5] Y. Sun et al. Pathsimsim: meta path-based top-k similarity search in heterogeneous information networks. In *VLDB*, 2011.
- [6] Y. Sun et al. Integrating meta-path selection with user-guided object clustering in heterogeneous information networks. In *SIGKDD*, pages 1348–1356, 2012.
